# Supplementary material for: Is there "Secret Sauce'' in Large Language Model Development?
Source: arXiv:2602.07238 source file (2026-05-03)
Supplement: Supplementary file 1 [file model_appendix.tex]

%\section*{Appendix: List of Models by Quarter}
%\noindent
%\textbf{Note:} This appendix lists all models used in the analysis, grouped by release quarter.

\subsection*{2023q1}
\begin{multicols}{3}
\begin{itemize}\setlength\itemsep{0pt}
  \item flan-ul2
  \item gpt-sw3-40b
  \item pythia-12b
  \item pythia-160m
  \item pythia-2.8b
  \item pythia-410m
  \item pythia-6.9b
\end{itemize}
\end{multicols}

\subsection*{2023q2}
\begin{multicols}{3}
\begin{itemize}\setlength\itemsep{0pt}
  \item RedPajama-INCITE-7B-Base
  \item RedPajama-INCITE-7B-Chat
  \item RedPajama-INCITE-Base-3B-v1
  \item RedPajama-INCITE-Chat-3B-v1
  \item Ziya-LLaMA-13B-v1
  \item dolly-v2-12b
  \item falcon-40b
  \item falcon-40b-instruct
  \item falcon-7b
  \item falcon-7b-instruct
  \item mpt-7b
\end{itemize}
\end{multicols}

\subsection*{2023q3}
\begin{multicols}{3}
\begin{itemize}\setlength\itemsep{0pt}
  \item LLaMA-2-7B-32K
  \item Llama-2-13b-chat-hf
  \item Llama-2-13b-hf
  \item Llama-2-70b-chat-hf
  \item Llama-2-70b-hf
  \item Llama-2-7b-chat-hf
  \item Llama-2-7b-hf
  \item phi-1
  \item phi-1\_5
  \item stablelm-3b-4e1t
\end{itemize}
\end{multicols}

\subsection*{2023q4}
\begin{multicols}{3}
\begin{itemize}\setlength\itemsep{0pt}
  \item Sheared-LLaMA-1.3B
  \item Sheared-LLaMA-2.7B
  \item Starling-LM-7B-alpha
  \item TinyLlama-1.1B-Chat-v1.0
  \item TinyLlama-1.1B-intermediate-step-1431k-3T
  \item Yi-34B
  \item Yi-34B-Chat
  \item Yi-6B
  \item Yi-6B-200K
  \item Yi-6B-Chat
  \item deepseek-llm-67b-chat
  \item deepseek-llm-7b-base
  \item deepseek-llm-7b-chat
  \item nucleus-22B-token-500B
  \item openchat\_3.5
  \item phi-2
  \item starcoder2-3b
  \item zephyr-7b-alpha
\end{itemize}
\end{multicols}

\subsection*{2024q1}
\begin{multicols}{3}
\begin{itemize}\setlength\itemsep{0pt}
  \item Claude-3-Opus
  \item Indic-gemma-2b-finetuned-sft-Navarasa-2.0
  \item Indic-gemma-7b-finetuned-sft-Navarasa-2.0
  \item Jamba-v0.1
  \item LLaMA-Pro-8B
  \item LLaMA-Pro-8B-Instruct
  \item Luminia-13B-v3
  \item MicroLlama
  \item Qwen1.5-0.5B
  \item Qwen1.5-0.5B-Chat
  \item Qwen1.5-1.8B
  \item Qwen1.5-1.8B-Chat
  \item Qwen1.5-14B
  \item Qwen1.5-14B-Chat
  \item Qwen1.5-4B
  \item Qwen1.5-4B-Chat
  \item Qwen1.5-72B-Chat
  \item Qwen1.5-7B
  \item Qwen1.5-7B-Chat
  \item RakutenAI-7B
  \item RakutenAI-7B-chat
  \item Staring-7B
  \item TinyLlama\_v1.1
  \item TinyMistral-248M-v3
  \item Yi-9B
  \item Yi-9B-200K
  \item bigyi-15b
  \item dbrx-instruct
  \item deepseek-moe-16b-base
  \item gemma-1.1-2b-it
  \item gemma-1.1-7b-it
  \item gemma-2b
  \item gemma-2b-orpo
  \item gemma-7b
  \item gemma-7b-it
  \item internlm2-1\_8b
  \item internlm2-chat-1\_8b
  \item stablelm-2-12b
  \item stablelm-2-1\_6b
  \item starcoder2-15b
  \item starcoder2-7b
\end{itemize}
\end{multicols}

\subsection*{2024q2}
\begin{multicols}{3}
\begin{itemize}\setlength\itemsep{0pt}
  \item Codestral-22B-v0.1
  \item Deepseek-V2-Chat
  \item Fox-1-1.6B
  \item GPT-4-Turbo
  \item Gemini-1.5-Flash
  \item Gemini-1.5-Pro
  \item Gemma-2-27B-it
  \item Gemma-2-9B-it
  \item Higgs-Llama-3-70B
  \item InstructLM-500M
  \item K2
  \item K2-Chat
  \item L3-8B-Lunaris-v1
  \item LLaMAntino-3-ANITA-8B-Inst-DPO-ITA
  \item Llama-3-70B-Orpo-v0.1
  \item Llama-3-Instruct-8B-SimPO
  \item Llama-3-SauerkrautLM-70b-Instruct
  \item Meta-Llama-3-70B
  \item Meta-Llama-3-70B-Instruct
  \item Meta-Llama-3-8B-Instruct
  \item MiniCPM-S-1B-sft-llama-format
  \item OLMo-1B-hf
  \item OLMo-7B-hf
  \item Phi-3-medium-128k-instruct
  \item Phi-3-medium-4k-instruct
  \item Phi-3-mini-128k-instruct
  \item Phi-3-mini-4k-instruct
  \item Phi-3-mini-4k-instruct-sa-v0.1
  \item Phi-3-small-128k-instruct
  \item Phi-3-small-8k-instruct
  \item Phi3-medium-4k
  \item Phi3-mini-4k
  \item Qwen-las-v0.1
  \item Qwen2-0.5B
  \item Qwen2-0.5B-Instruct
  \item Qwen2-57B-A14B
  \item Qwen2-57B-A14B-Instruct
  \item Qwen2-72B
  \item Qwen2-72B-Instruct
  \item Qwen2-7B-Instruct
  \item Reka 3
  \item SauerkrautLM-1.5b
  \item SauerkrautLM-Phi-3-medium
  \item StarFusion-alpha1
  \item Tess-v2.5-Phi-3-medium-128k-14B
  \item Yi-1.5-34B
  \item Yi-1.5-34B-32K
  \item Yi-1.5-34B-Chat
  \item Yi-1.5-34B-Chat-16K
  \item Yi-1.5-6B
  \item Yi-1.5-6B-Chat
  \item Yi-1.5-9B-Chat
  \item Yi-large
  \item YiSM-34B-0rn
  \item c4ai-command-r-plus
  \item calme-2.1-phi3-4b
  \item calme-2.2-phi3-4b
  \item calme-2.3-phi3-4b
  \item codegemma-1.1-2b
  \item deepseek-llm-7b-chat-sa-v0.1
  \item dictalm2.0
  \item dictalm2.0-instruct
  \item dolphin-2.9.1-llama-3-70b
  \item dolphin-2.9.1-yi-1.5-34b
  \item dolphin-2.9.2-qwen2-72b
  \item dolphin-2.9.3-Yi-1.5-34B-32k
  \item falcon-11B
  \item fietje-2
  \item fietje-2-instruct
  \item gemma-2-27b
  \item gemma-2-27b-it
  \item gemma-2-9b
  \item gemma-2-9b-it
  \item gemma-mling-7b
  \item granite-7b-base
  \item granite-7b-instruct
  \item leniachat-gemma-2b-v0
  \item magnum-v1-72b
  \item openbuddy-yi1.5-34b-v21.3-32k
  \item qwen1.5-7b-chat-sa-v0.1
  \item suzume-llama-3-8B-multilingual
  \item zephyr-orpo-141b-A35b-v0.1
\end{itemize}
\end{multicols}

\subsection*{2024q3}
\begin{multicols}{3}
\begin{itemize}\setlength\itemsep{0pt}
  \item 1.5-Pints-16K-v0.1
  \item 1.5-Pints-2K-v0.1
  \item 10PRYMMAL-3B-slerp
  \item 2PRYMMAL-Yi1.5-6B-SLERP
  \item AMD-Llama-135m
  \item Astra-v1-12B
  \item Athena-gemma-2-2b-it
  \item Bielik-11B-v2
  \item Bielik-11B-v2.0-Instruct
  \item Bielik-11B-v2.1-Instruct
  \item Bielik-11B-v2.2-Instruct
  \item Bielik-11B-v2.3-Instruct
  \item BigQwen2.5-52B-Instruct
  \item BigQwen2.5-Echo-47B-Instruct
  \item Bio-Medical-Llama-3-8B
  \item CantoneseLLMChat-v0.5
  \item Chronos-Gold-12B-1.0
  \item DCLM-7B
  \item Dans-Instruct-CoreCurriculum-12b-ChatML
  \item Darkens-8B
  \item DeepSeek-Chat-V2\_5
  \item DeepSeek-Coder-V2-Instruct
  \item EXAONE-3.0-7.8B-Instruct
  \item Einstein-v8-Llama3.2-1B
  \item Explore\_Llama-3.1-8B-Inst
  \item FuseChat-7B-v2.0
  \item GPT-4o-mini
  \item Gemma-2-2B-it
  \item Gemma2-9B-IT-Simpo-Infinity-Preference
  \item Grok-2
  \item Josiefied-Qwen2.5-1.5B-Instruct-abliterated-v1
  \item Josiefied-Qwen2.5-7B-Instruct-abliterated-v2
  \item Josiefied-Qwen2.5-7B-Instruct-abliterated-v2
  \item LLaMA-2-vicuna-7b-slerp
  \item Llama-3-8B-ProLong-512k-Base
  \item Llama-3-8B-ProLong-512k-Instruct
  \item Llama-3-8B-ProLong-64k-Base
  \item Llama-3-8B-ProLong-64k-Instruct
  \item Llama-3.1-405B
  \item Llama-3.1-405B-Instruct
  \item Llama-3.1-70B
  \item Llama-3.1-70B-Instruct
  \item Llama-3.1-8B
  \item Llama-3.1-8B-MagPie-Ultra
  \item Llama-3.2-1B
  \item Llama-3.2-1B-Instruct
  \item Llama-3.2-1B-Instruct
  \item Llama-3.2-3B
  \item Llama-3.2-3B-Instruct
  \item Llama-3.2-SUN-2.4B-checkpoint-26000
  \item Llama-3.2-SUN-2.4B-checkpoint-34800
  \item Llama-3.2-SUN-2.4B-v1.0.0
  \item Llama-3.2-SUN-2.5B-chat
  \item Llama-eus-8B
  \item Llama3.1-8B-Cobalt
  \item LlamaExecutor-8B-3.0.5
  \item Mathstral-7B-v0.1
  \item Minitron-4B-Base
  \item Minitron-8B-Base
  \item Mistral-Large-Instruct-2407
  \item Mistral-NeMo-Minitron-8B-Base
  \item Mistral-NeMo-Minitron-8B-Chat
  \item Mistral-NeMo-Minitron-Upscale-v1
  \item Mistral-NeMo-Minitron-Upscale-v2
  \item Mistral-Nemo-Base-2407
  \item Mistral-Nemo-Instruct-2407
  \item Mistral-Small-instruct
  \item NepaliGPT-2.0
  \item OLMoE-1B-7B-0924
  \item OLMoE-1B-7B-0924-Instruct
  \item Odin-9B
  \item OpenMath2-Llama3.1-8B
  \item PRYMMAL-6B-slerp
  \item Pantheon-RP-1.5-12b-Nemo
  \item Pantheon-RP-1.6-12b-Nemo
  \item Pantheon-RP-1.6-12b-Nemo-KTO
  \item Phi-1\_5-Instruct-v0.1
  \item Phi-3.5-MoE-instruct
  \item Phi-3.5-mini-instruct
  \item Qwen2-0.5B-Abyme
  \item Qwen2-72B-Chat
  \item Qwen2.5-0.5B
  \item Qwen2.5-0.5B-Instruct
  \item Qwen2.5-1.5B
  \item Qwen2.5-1.5B-Instruct
  \item Qwen2.5-14B
  \item Qwen2.5-14B-Gutenberg-1e-Delta
  \item Qwen2.5-14B-Instruct
  \item Qwen2.5-32B
  \item Qwen2.5-32B-Instruct
  \item Qwen2.5-3B
  \item Qwen2.5-3B-Instruct
  \item Qwen2.5-72B
  \item Qwen2.5-72B-Instruct
  \item Qwen2.5-7B
  \item Qwen2.5-7B-Instruct
  \item Qwen2.5-7B-Instruct-Uncensored
  \item Qwen2.5-7B-Instruct-abliterated
  \item Qwen2.5-7B-Instruct-abliterated-v2
  \item Qwen2.5-95B-Instruct
  \item Qwen2.5-Coder-7B
  \item Qwen2.5-Coder-7B-Instruct
  \item Qwen2.5-Lumen-14B
  \item Qwen2.5-Math-7B
  \item RYS-Llama-3.1-8B-Instruct
  \item RYS-Phi-3-medium-4k-instruct
  \item RYS-XLarge-base
  \item Rombos-LLM-V2.5-Qwen-32b
  \item Rombos-LLM-V2.5-Qwen-72b
  \item SmolLM-1.7B
  \item SmolLM-1.7B-Instruct
  \item SmolLM-135M
  \item SmolLM-135M-Instruct
  \item SmolLM-360M
  \item SmolLM-360M-Instruct
  \item T.E-8.1
  \item Tor-8B
  \item Trinity-2-Codestral-22B
  \item Trinity-2-Codestral-22B-v0.2
  \item Yi-1.5-9B-Chat-abliterated
  \item Yibuddy-35B
  \item Yislerp2-34B
  \item calme-2.1-phi3.5-4b
  \item calme-2.1-qwen2.5-72b
  \item calme-2.2-qwen2-72b
  \item calme-2.2-qwen2.5-72b
  \item calme-2.3-qwen2-72b
  \item dolphin-2.9.3-mistral-nemo-12b
  \item dolphin-2.9.4-gemma2-2b
  \item falcon-mamba-7b
  \item gemma-2-27b-it-SimPO-37K
  \item gemma-2-27b-it-SimPO-37K-100steps
  \item gemma-2-2b
  \item gemma-2-2b-it
  \item gemma-2-2b-jpn-it
  \item gemma-2-9B-MOTH
  \item gemma-2-9b-it-DPO
  \item gemma-2-9b-it-SimPO
  \item gemma-2-9b-it-WPO-HB
  \item gemma2-gutenberg-27B
  \item h2o-danube3-4b-base
  \item h2o-danube3-4b-chat
  \item h2o-danube3-500m-chat
  \item internlm2\_5-20b-chat
  \item lambda-gemma-2-9b-dpo
  \item lambda-qwen2.5-14b-dpo-test
  \item lambda-qwen2.5-32b-dpo-test
  \item ldm\_soup\_Llama-3.1-8B-Inst
  \item llama-3-8b-instruct-gapo-v2-bert-f1-beta10-gamma0.3-lr1.0e-6-1minus-rerun
  \item llama-3-8b-instruct-gapo-v2-bert\_f1-beta10-gamma0.3-lr1.0e-6-scale-log
  \item llama-3-8b-instruct-gapo-v2-bert\_p-beta10-gamma0.3-lr1.0e-6-scale-log
  \item llama-3-8b-instruct-gapo-v2-rouge2-beta10-1minus-gamma0.3-rerun
  \item llama-3-8b-instruct-gapo-v2-rouge2-beta10-gamma0.3-lr1.0e-6-scale-log
  \item llama-3-8b-instruct-gapo-v2-rougeL-beta10-gamma0.3-lr1.0e-6-scale-log
  \item magistrate-3.2-3b-base
  \item magnum-v2-12b
  \item magnum-v3-34b
  \item magnum-v3-9b-customgemma2
  \item merge-test
  \item openbuddy-llama3.1-8b-v22.2-131k
  \item phi-2-instruct-apo
  \item phi-2-instruct-v0.1
  \item qwen2.5-reinstruct-alternate-lumen-14B
  \item salamandra-7b
  \item salamandra-7b-instruct
  \item tangled-llama-pints-1.5b-v0.1-instruct
  \item tangled-llama-pints-1.5b-v0.2-instruct
\end{itemize}
\end{multicols}

\subsection*{2024q4}
\begin{multicols}{3}
\begin{itemize}\setlength\itemsep{0pt}
  \item 13\_outOf\_32\_pruned\_layers\_llama3.1-8b
  \item 2\_PRYMMAL-ECE-2B-SLERP-V1
  \item ArlowGPT-8B
  \item Athena-1-3B
  \item BgGPT-Gemma-2-27B-IT-v1.0
  \item Chocolatine-14B-Instruct-DPO-v1.3
  \item Claude 3.5 Sonnet
  \item DRT-o1-14B
  \item DRT-o1-7B
  \item Dans-PersonalityEngine-V1.1.0-12b
  \item Dans-PersonalityEngine-v1.0.0-8b
  \item Deepseek-V3
  \item Deepthink-Reasoning-7B
  \item Dolphin3.0-Llama3.1-8B
  \item Dolphin3.0-Llama3.2-1B
  \item Dolphin3.0-Qwen2.5-0.5B
  \item ECE-PRYMMAL-0.5B-FT-V3-MUSR
  \item ECE-PRYMMAL-0.5B-FT-V4-MUSR
  \item ECE-PRYMMAL0.5B-Youri
  \item EVA-Qwen2.5-14B-v0.2
  \item EVA-Qwen2.5-72B-v0.2
  \item EXAONE-3.5-2.4B-Instruct
  \item EXAONE-3.5-32B-Instruct
  \item EXAONE-3.5-7.8B-Instruct
  \item Explore\_Llama-3.2-1B-Inst
  \item Explore\_Llama-3.2-1B-Inst\_v1
  \item Explore\_Llama-3.2-1B-Inst\_v1.1
  \item Eyas-17B-Instruct
  \item Falcon3-10B-Base
  \item Falcon3-10B-Instruct
  \item Falcon3-1B-Base
  \item Falcon3-1B-Instruct
  \item Falcon3-2x10B-MoE-Instruct
  \item Falcon3-3B-Base
  \item Falcon3-3B-Instruct
  \item Falcon3-7B-Base
  \item Falcon3-7B-Instruct
  \item Falcon3-Mamba-7B-Base
  \item Falcon3-Mamba-7B-Instruct
  \item Falcon3-MoE-2x7B-Insruct
  \item Falcon3Slerp1-10B
  \item FalconSlerp1-7B
  \item FalconSlerp3-7B
  \item FalconThink3-10B-IT
  \item FinancialAdvice-Qwen2.5-7B
  \item Fusion-14B-Instruct
  \item Fusion2-14B-Instruct
  \item GPT-4o (2024-11-20)
  \item GPT-NEO-1.3B-wiki
  \item GPT-o1
  \item Gemini-2.0-Flash-exp
  \item Humanish-LLama3-8B-Instruct
  \item Humanish-Qwen2.5-7B-Instruct
  \item Hunyuan-Large
  \item Hymba-1.5B-Base
  \item Hymba-1.5B-Instruct
  \item INTELLECT-1
  \item INTELLECT-1-Instruct
  \item Josiefied-Qwen2.5-14B-Instruct-abliterated-v4
  \item L3.1-Pneuma-8B
  \item LLAMA\_Harsha\_8\_B\_ORDP\_10k
  \item LLaMa-3.1-Instruct-Interleaved-Zeroed-13B
  \item LLaMa-3.2-Instruct-JankMixBread-v0.1-3B
  \item Linkbricks-Horizon-AI-Avengers-V1-32B
  \item Linkbricks-Horizon-AI-Korean-Superb-27B
  \item Linkbricks-Horizon-AI-Superb-27B
  \item Llama-3.1-8B-Instruct-Zeus
  \item Llama-3.1-8B-Open-SFT
  \item Llama-3.1-8B-OpenO1-SFT-v0.1
  \item Llama-3.1-8B-paraphrase-type-generation-apty-ipo
  \item Llama-3.1-8B-paraphrase-type-generation-apty-sigmoid
  \item Llama-3.1-8B-paraphrase-type-generation-etpc
  \item Llama-3.1-Argunaut-1-8B-SFT
  \item Llama-3.1-MedIT-SUN-8B
  \item Llama-3.1-Tulu-3-70B-SFT
  \item Llama-3.1-Tulu-3-8B-SFT
  \item Llama-3.1\_OpenScholar-8B
  \item Llama-3.2-1B-Instruct-gptqmodel-4bit-vortex-v1
  \item Llama-3.2-1B-SPIN-iter0
  \item Llama-3.2-1B-SPIN-iter1
  \item Llama-3.2-1B-SPIN-iter2
  \item Llama-3.2-1B-SPIN-iter3
  \item Llama-3.2-Instruct-3B-TIES
  \item Llama-3.2-SUN-1B-Instruct
  \item Llama-3.2-SUN-1B-chat
  \item Llama-3.2-SUN-HDIC-1B-Instruct
  \item Llama-3.3-70B-Instruct
  \item Llama-Deepsync-1B
  \item Llama-Nephilim-Metamorphosis-v2-8B
  \item Llama-TI-8B
  \item Llama-TI-8B-Instruct
  \item Llama3.1-8B-PlumChat
  \item Llama3.1-8B-PlumCode
  \item Llama3.1-8B-PlumMath
  \item Marco-01-slerp1-7B
  \item Marco-o1
  \item MedIT-Mesh-3B-Instruct
  \item MiniQwenMathExpert-ECE-PRYMMAL-Martial
  \item Ministral-8B-Instruct-2410
  \item Ministral-8B-Instruct-2410-HF
  \item Mistral-NeMo-Minitron-8B-Instruct
  \item Mistral-NeMo-Minitron-Upscale-v3
  \item MoE-Girl-1BA-7BT
  \item MobileLLM-125M-HF
  \item N3N\_Llama-3.1-8B-Instruct\_1028\_0216
  \item Neos-Gemma-2-9b
  \item Neos-Llama-3.1-8B
  \item Neos-Phi-3-14B-v0.1
  \item OLMo-2-1124-7B-Instruct
  \item PARM-V1.5-base-QwQ-Qwen-2.5-o1-3B
  \item PathFinderAI2.0
  \item PathFinderAi3.0
  \item PathfinderAI
  \item PeiYangMe-0.5
  \item PeiYangMe-0.7
  \item QAIMath-Qwen2.5-7B-TIES
  \item Quill-v1
  \item QwQ-32B-Preview
  \item QwQ-LCoT-3B-Instruct
  \item QwQ-LCoT-7B-Instruct
  \item Qwen-7B-nerd-uncensored-v1.0
  \item Qwen-Megumin
  \item Qwen2.5-0.5B-SFT
  \item Qwen2.5-0.5B-SFT-1e-4
  \item Qwen2.5-0.5B-SFT-1e-4-2ep
  \item Qwen2.5-0.5B-SFT-1e-4-3ep
  \item Qwen2.5-0.5B-SFT-1e-4-5ep
  \item Qwen2.5-0.5B-SFT-1e-5
  \item Qwen2.5-0.5B-SFT-1e-5-2ep
  \item Qwen2.5-0.5B-SFT-1e-5-3ep
  \item Qwen2.5-0.5B-SFT-1e-5-5ep
  \item Qwen2.5-0.5B-SFT-2e-4
  \item Qwen2.5-0.5B-SFT-2e-4-2ep
  \item Qwen2.5-0.5B-SFT-2e-4-3ep
  \item Qwen2.5-0.5B-SFT-2e-4-5ep
  \item Qwen2.5-0.5B-SFT-2e-5
  \item Qwen2.5-0.5B-SFT-2e-5-2ep
  \item Qwen2.5-0.5B-SFT-2e-5-3ep
  \item Qwen2.5-0.5B-SFT-2e-5-5ep
  \item Qwen2.5-0.5B-SFT-5e-5
  \item Qwen2.5-0.5B-SFT-5e-5-2ep
  \item Qwen2.5-0.5B-SFT-5e-5-3ep
  \item Qwen2.5-0.5B-SFT-5e-5-5ep
  \item Qwen2.5-0.5B-SFT-7e-5
  \item Qwen2.5-0.5B-SFT-7e-5-2ep
  \item Qwen2.5-0.5B-SFT-7e-5-3ep
  \item Qwen2.5-0.5B-SFT-7e-5-5ep
  \item Qwen2.5-14B-Instruct-abliterated-v2
  \item Qwen2.5-14B-Wernickev3
  \item Qwen2.5-32B-Instruct-abliterated-v2
  \item Qwen2.5-3B-RP-Mix
  \item Qwen2.5-72B-Instruct-abliterated
  \item Qwen2.5-72B-Instruct-abliterated
  \item Qwen2.5-7B-Anvita
  \item Qwen2.5-7B-Instruct-Fusion
  \item Qwen2.5-7B-della-test
  \item Qwen2.5-7B-minperplexity-2
  \item Qwen2.5-7B-nerd-uncensored-v0.9
  \item Qwen2.5-7B-nerd-uncensored-v1.0
  \item Qwen2.5-7B-nerd-uncensored-v1.1
  \item Qwen2.5-7B-nerd-uncensored-v1.2
  \item Qwen2.5-7B-nerd-uncensored-v1.3
  \item Qwen2.5-7B-nerd-uncensored-v1.4
  \item Qwen2.5-7B-nerd-uncensored-v1.5
  \item Qwen2.5-7B-nerd-uncensored-v1.7
  \item Qwen2.5-7B-nerd-uncensored-v1.8
  \item Qwen2.5-7B-olm-v1.0
  \item Qwen2.5-7B-olm-v1.1
  \item Qwen2.5-Coder-14B
  \item Qwen2.5-Coder-14B-Instruct
  \item Qwen2.5-Coder-32B
  \item Qwen2.5-Coder-32B-Instruct
  \item Qwen2.5-Coder-7B-Instruct-20241106
  \item Qwen2.5-Gutenberg-Doppel-14B
  \item Qwen2.5-Math-14B-Instruct-Pro
  \item Qwen2.5-Ultimate-14B-Instruct
  \item QwenMosaic-7B
  \item Qwentile2.5-32B-Instruct
  \item Qwenvergence-14B-v6-Prose
  \item RA\_Reasoner
  \item RQwen-v0.1
  \item Rombos-LLM-V2.5-Qwen-14b
  \item Rombos-LLM-V2.5-Qwen-3b
  \item Rombos-LLM-V2.5-Qwen-7b
  \item Rombos-LLM-V2.5.1-Qwen-3b
  \item Rombos-LLM-V2.6-Qwen-14b
  \item Rombos-Qwen2.5-7B-Inst-BaseMerge-TIES
  \item SASTRI\_1\_9B
  \item SKY-Ko-Llama3.1-8B-lora
  \item SKY-Ko-Llama3.2-1B-lora-epoch3
  \item SKY-Ko-Llama3.2-1B-lora-epoch5
  \item SKY-Ko-Llama3.2-1B-lora-v2-epoch3
  \item SKY-Ko-Llama3.2-1B-lora-v2-epoch5
  \item Saba1-7B
  \item SauerkrautLM-v2-14b-DPO
  \item SauerkrautLM-v2-14b-SFT
  \item Skywork-Reward-Gemma-2-27B-v0.2
  \item SmallThinker-3B-Preview
  \item SmolLM2-1.7B
  \item SmolLM2-1.7B-Instruct
  \item SmolLM2-1.7B-Merged
  \item SmolLM2-135M
  \item SmolLM2-135M-Instruct
  \item SmolLM2-135M-Merged
  \item SmolLM2-360M
  \item SmolLM2-360M-Instruct
  \item SmolLM2-360M-Merged
  \item SmolLM2-MedIT-Upscale-2B
  \item SmolTulu-1.7b-Instruct
  \item SmolTulu-1.7b-it-v0
  \item Sphinx2.0
  \item StructuredThinker-v0.3-MoreStructure
  \item SuperNova-Medius
  \item Teleut-7b
  \item TheBeagle-v2beta-32B-MGS
  \item Tsunami-0.5-7B-Instruct
  \item Tsunami-0.5x-7B-Instruct
  \item Tsunami-1.0-14B-Instruct
  \item Tsunami-1.0-7B-Instruct
  \item Virtuoso-Small
  \item Yi-Lightning
  \item autotrain-0tmgq-5tpbg
  \item autotrain-llama32-1b-finetune
  \item aya-expanse-32b
  \item bacon\_and\_food
  \item c4ai-command-r7b-12-2024
  \item calme-3.1-baguette-3b
  \item calme-3.1-instruct-3b
  \item calme-3.1-llamaloi-3b
  \item calme-3.2-baguette-3b
  \item calme-3.2-instruct-3b
  \item calme-3.3-baguette-3b
  \item calme-3.3-instruct-3b
  \item cp2024
  \item cp2024-instruct
  \item cybertron-v4-qw7B-MGS
  \item cybertron-v4-qw7B-UNAMGS
  \item falcon3-ultraset
  \item franqwenstein-35b
  \item gemma-2-2b-ORPO-jpn-it-abliterated-18
  \item gemma-2-2b-ORPO-jpn-it-abliterated-18-merge
  \item gemma-2-2b-jpn-it-abliterated-17
  \item gemma-2-2b-jpn-it-abliterated-17-18-24
  \item gemma-2-2b-jpn-it-abliterated-17-ORPO
  \item gemma-2-2b-jpn-it-abliterated-18
  \item gemma-2-2b-jpn-it-abliterated-18-ORPO
  \item gemma-2-2b-jpn-it-abliterated-24
  \item gen-inst-1
  \item granite-3.0-1b-a400m-base
  \item granite-3.0-1b-a400m-instruct
  \item granite-3.0-2b-base
  \item granite-3.0-2b-instruct
  \item granite-3.0-3b-a800m-base
  \item granite-3.0-3b-a800m-instruct
  \item granite-3.0-8b-base
  \item granite-3.0-8b-instruct
  \item granite-3.1-1b-a400m-base
  \item granite-3.1-1b-a400m-instruct
  \item granite-3.1-2b-base
  \item granite-3.1-2b-instruct
  \item granite-3.1-8b-base
  \item granite-3.1-8b-instruct
  \item huihui-ai-abliterated-Qwen2.5-32B-Inst-BaseMerge-TIES
  \item intelligence-cod-rag-7b-v3
  \item jeffmeloy\_Qwen2.5-7B-minperplexity-1
  \item lareneg3B-ECE-PRYMMAL-Martial
  \item magistrate-3.2-3b-it
  \item miscii-14b-1028
  \item model-3
  \item naps-gemma-2-27b-v-0.1.0
  \item naps-gemma-2-27b-v0.1.0
  \item naps-llama-3\_1\_instruct-v0.6.0
  \item notHumpback-M0
  \item notHumpback-M1
  \item openbuddy-qwen2.5llamaify-7b-v23.1-200k
  \item orca\_mini\_v8\_1\_70b
  \item orca\_mini\_v9\_1\_1B-Instruct
  \item orca\_mini\_v9\_2\_70b
  \item orca\_mini\_v9\_5\_1B-Instruct\_preview
  \item oxy-1-small
  \item pancho-v1-qw25-3B-UNAMGS
  \item phi-4
  \item phi-4-abliterated
  \item pruned10-llama-3.2-3B
  \item pruned20-llama-1b
  \item pruned20-llama-3.2-3b
  \item pruned40-llama-1b
  \item pruned40-llama-3.2-1B
  \item pruned40-llama-3.2-3b
  \item pruned60-llama-1b
  \item pruned60-llama-3.2-3b
  \item qwen-carpmuscle-r-v0.3
  \item raspberry-3B
  \item reasoning-1-1k-demo
  \item rombos\_Replete-Coder-Llama3-8B
  \item shuttle-3
  \item smallcp2024
  \item smol-360m-ft
  \item ultiima-32B
  \item zetasepic-abliteratedV2-Qwen2.5-32B-Inst-BaseMerge-TIES
\end{itemize}
\end{multicols}

\subsection*{2025q1}
\begin{multicols}{3}
\begin{itemize}\setlength\itemsep{0pt}
  \item 0x-lite
  \item 70B-L3.3-Cirrus-x1
  \item AceCoder-Qwen2.5-7B-Ins-Rule
  \item AceCoder-Qwen2.5-Coder-7B-Base-Rule
  \item Anemoi-3B
  \item Apollo\_v2-32B
  \item BBA99
  \item BBAI\_7B\_KoenQwenDyan
  \item BBAI\_7B\_Qwen2.5koen
  \item BBALAW1.0
  \item BBALAW1.61
  \item Barcenas-10b
  \item Barcenas-14b-phi-4
  \item Barcenas-14b-phi-4-v2
  \item Bellatrix-Tiny-1B-v2
  \item Bifrost
  \item Bio-Medical-3B-CoT-012025
  \item Blossom-V6-14B
  \item Blossom-V6-7B
  \item Calcium-Opus-14B-Elite
  \item Calcium-Opus-14B-Elite2
  \item Calcium-Opus-14B-Elite3
  \item Calcium-Opus-14B-Elite4
  \item Calcium-Opus-14B-Merge
  \item Calcium-Opus-20B-v1
  \item Chirp-01
  \item Coder-GRPO-3B
  \item CogitoZ
  \item Confucius-o1-14B
  \item DeepPhi-3.5-mini-instruct
  \item DeepSauerHuatuoSkywork-R1-o1-Llama-3.1-8B
  \item DeepSeek-R1
  \item DeepThinkers-Phi4
  \item Deepthink-Llama-3-8B-Preview
  \item Deepthink-Reasoning-14B
  \item Dobby-Mini-Leashed-Llama-3.1-8B
  \item Dobby-Mini-Unhinged-Llama-3.1-8B
  \item Doubao-1.5-Pro
  \item EVA-abliterated-TIES-Qwen2.5-14B
  \item Epimetheus-14B-Axo
  \item Falcon3-8B-Franken-Basestruct
  \item Flashlight-v1.0
  \item Flashlight-v1.1
  \item GPT-4.5
  \item Gauss-Opus-14B-R999
  \item Gemini-2.0-Pro
  \item Gemma-3-1B-it
  \item Gemma-3-27B-it
  \item Gemma-3-4B-it
  \item Gemma2-9B-AdvancedFuse
  \item Gilgamesh-72B
  \item Grok3-Beta
  \item HF\_TOKEN
  \item Hunyuan-T1
  \item HunyuanTurboS
  \item IE-cont-Llama3.1-8B
  \item ILAB-Merging-3B-V2
  \item Internlm3-8B-Instruct
  \item Kyro-n1-3B
  \item Kyro-n1-7B
  \item L3.1-8b-RP-Ink
  \item Llama-3.1-8B-GRPO-Instruct
  \item Llama-3.1-8B-R1-v0.1
  \item Llama-3.1-8B-SFT-GRPO-Instruct
  \item Llama-3.2-3B-Khelavaster
  \item Llama-Express.1-Math
  \item Llama3.2.1B.0.01-First
  \item Llama3.2.1B.0.01-Last
  \item Llama3.2.1B.0.1-First
  \item Llama3.2.1B.0.1-Last
  \item Llama3.2.1B.BaseFiT
  \item Llama3.3-70B-CogniLink
  \item LwQ-10B-Instruct
  \item MawaredT1
  \item Megatron-Opus-14B-2.0
  \item Megatron-Opus-14B-2.1
  \item MiniMax-Text-01
  \item MiniThinky-1B-Llama-3.2
  \item MiniThinky-v2-1B-Llama-3.2
  \item Mistral-3.1-Small
  \item Nexuim-R1-7B-Instruct
  \item NxMobileLM-1.5B-SFT
  \item OpenCognito-r1
  \item OpenCognito-r2
  \item OpenThinker-7B
  \item Phi-4-Empathetic
  \item Phi-4-Math-IO
  \item Phi-4-Model-Stock
  \item Phi-4-QwQ
  \item Phi-4-mini-UNOFFICAL
  \item Phi-4-mini-instruct
  \item Phi-4-o1
  \item Phi-Line\_14B
  \item Phi-lthy4
  \item Phi4.Turn.R1Distill.16bit
  \item Precis-1B-Instruct
  \item Qmerft
  \item QwEnlarge-16B-Instruct
  \item QwOwO-7B-V1
  \item QwQ-32B
  \item QwQ-LCoT-14B-Conversational
  \item QwQ-LCoT2-7B-Instruct
  \item QwQ-MathOct-7B
  \item Qwen-2.5-14B-Hindi-Custom-Instruct
  \item Qwen2.5-1.5B-DeepSeek-R1-Instruct
  \item Qwen2.5-14B-1M-YOYO-V3
  \item Qwen2.5-14B-Instruct
  \item Qwen2.5-14B-Instruct-1M
  \item Qwen2.5-14B-YOYO-V4
  \item Qwen2.5-14B-YOYO-V4-p1
  \item Qwen2.5-14B-YOYO-V4-p2
  \item Qwen2.5-14B-it-restore
  \item Qwen2.5-3B-Infinity-Instruct-0625
  \item Qwen2.5-4B
  \item Qwen2.5-7B-Fuse-Exp
  \item Qwen2.5-7B-Instruct-1M
  \item Qwen2.5-7B-Instruct-Merge-Stock-v0.1
  \item Qwen2.5-7B-Instruct-QwQ-v0.1
  \item Qwen2.5-7B-MS-Destroyer
  \item Qwen2.5-7B-it-restore
  \item Qwen2.5-7B-olm-v1.2
  \item Qwen2.5-7B-olm-v1.3
  \item Qwen2.5-7B-olm-v1.4
  \item Qwen2.5-7B-olm-v1.5
  \item Qwen2.5-Max
  \item Qwen2.5-THREADRIPPER-Small
  \item QwenQwen2.5-7B-IT
  \item QwenQwen2.5-7B-IT-Dare
  \item Qwen\_0.5-DPO\_5e-7-1ep\_0alp\_0lam
  \item Rombo-LLM-V2.5-Qwen-7b
  \item SJT-2B
  \item SKY-Ko-Llama3.1-8B-lora-epoch1
  \item SKY-Ko-Qwen2.5-3B-Instruct
  \item SKY-Ko-Qwen2.5-7B-Instruct-SFT-step-15000
  \item SKY-Ko-Qwen2.5-7B-Instruct-SFT-step-5000
  \item SakalFusion-7B-Alpha
  \item SkyThought-T1
  \item SmolLM2-CoT-360M
  \item Sombrero-Opus-14B-Sm1
  \item Sombrero-Opus-14B-Sm2
  \item Sombrero-Opus-14B-Sm5
  \item SuperThoughts-CoT-14B-16k-o1-QwQ
  \item Superthoughts-lite-1.8B-experimental-o1
  \item Superthoughts-lite-v1
  \item Taurus-Opus-7B
  \item Test\_StealthThinker
  \item TethysAI\_Base\_Reasoning
  \item Thinker-SmolLM2-135M-Instruct-Reasoning
  \item Viper-Coder-HybridMini-v1.3
  \item Virtuoso-Lite
  \item Virtuoso-Small-v2
  \item WebMind-7B-v0.1
  \item Xwen-7B-Chat
  \item ZYH-LLM-Qwen2.5-14B
  \item ZYH-LLM-Qwen2.5-14B-V3
  \item ZYH-LLM-Qwen2.5-14B-V4
  \item Zurich-14B-GCv2-5m
  \item chimera-beta-test2-lora-merged
  \item coolqwen-3b-it
  \item falcon3-10b-tensopolis-v1
  \item falcon3-10b-tensopolis-v2
  \item frqwen2.5-from7b-duable4layers-it
  \item frqwen2.5-from7b-it
  \item gemma-2-2b-it
  \item gemma-2-9b-it
  \item gemma-2-9b-it-chinese-kyara
  \item granite-3.2-8b-instruct
  \item helium-1-preview-2b
  \item jessi-v0.1-qwen2.5-7b-instruct
  \item jessi-v0.2-falcon3-7b-instruct
  \item jessi-v0.3-falcon3-7b-instruct
  \item jessi-v0.4-falcon3-7b-instruct
  \item jessi-v0.5-falcon3-7b-instruct
  \item jessi-v0.6-falcon3-7b-instruct
  \item li-14b-v0.4
  \item light-3B
  \item light-3b-beta
  \item light-7b-beta
  \item mistral-small-2501-tensopolis-v1
  \item mita-gen3-7b-2-26-2025
  \item moremerge
  \item openbuddy-falcon3-10b-v24.2-131k
  \item orca\_mini\_phi-4
  \item orca\_mini\_v9\_2\_14B
  \item orca\_mini\_v9\_4\_70B
  \item orca\_mini\_v9\_5\_1B-Instruct
  \item orca\_mini\_v9\_6\_1B-Instruct
  \item orca\_mini\_v9\_7\_1B-Instruct
  \item phi-4
  \item phi-4-25b
  \item phi-4-bnb-4bit
  \item phi-4-tensopolis-v1
  \item phi-4-unsloth-bnb-4bit
  \item qwen2.5-14b-tensopolis-v1
  \item qwen2.5-7b-cabs-v0.1
  \item qwen2.5-7b-cabs-v0.2
  \item qwen2.5-7b-cabs-v0.3
  \item qwen2.5-7b-cabs-v0.4
  \item qwen2.5-7b-tensopolis-v1
  \item qwen2.5-7b-tensopolis-v2
  \item qwen2.5-with-lora-think-3b-it
  \item qwmer
  \item sft-s1-qwen-0.5b
  \item smollm2-135M\_pretrained\_200k\_fineweb\_uncovai\_human\_removed
  \item smollm2-135M\_pretrained\_200k\_fineweb\_uncovai\_selected
  \item smollm2-360M-sft\_SmallThoughts
  \item smollm2\_pretrained\_200k\_fineweb
  \item t1-3B
  \item tinymistral\_950m
  \item trd-7b-it
  \item ud-14b
  \item ultiima-14B
  \item ultiima-72B
\end{itemize}
\end{multicols}
